# Supplementary material for: New Oracle-Efficient Algorithms for Private Synthetic Data Release
Source: arXiv:2007.05453 source file (2020-07-10)
Supplement: Supplementary file 1 [file appendix0.tex]

\newpage

\appendix

\section{Differential Privacy Tools}\label{appendix:A}

\begin{definition} A mechanism $M:\cX \rightarrow R$ satisfies $(\eps, \delta)$-differential privacy if for every $S\subset R$ and for all neighboring datasets $D,D'\in \cX$, the following holds:
$$\pr{M(D) \in S} \leq e^{\eps}\pr{M(D') \in S} + \delta$$
\end{definition}
\begin{definition}[Sensitivity]\label{def:sensitivity} The sensitivity of a function $f$ with range $R$ is

$$\Delta_f := \max_{D, D': |D \triangle D'| = 1, r \in R} |f(D, r) - f(D', r)|. $$
\end{definition}
\begin{definition}[Linear threshold functions]
A linear threshold function $\phi_p: \cX \rightarrow \{0,1\}$, is a linear mapping defined by a real valued set $P$ and vector coefficient $\phi$. With
\[
\phi_p(x) =
\begin{cases}
1 & \text{if } \inner{\phi}{x} \in P \\
0 & \text{otherwise }
\end{cases}
\]
\end{definition}

\begin{definition}[Statistical linear queries]
Given as predicate a linear threshold function $\phi$, the linear query $q_\phi: \cX^n \rightarrow [0,1]$ is defined by
$$q_\phi(D) = \frac{\sum_{x\in D} \phi(x)}{|D|}$$
\end{definition}

\begin{theorem}[Advanced Composition]
A set of $k$ mechanisms $\cM_1, \ldots \cM_k$ where each $\cM_k$ is $\epsilon_k$ -differentially private. Satisfies $(\epsilon', \delta)$-differential privacy  under $k$-fold adaptive composition for:
$$\epsilon'= \sum_{i=1}^k \epsilon_i(e^{\epsilon_i}-1) + \sqrt{\left( \sum_{i=1}^k \epsilon_i^2 \right) \ln\left( \frac{1}{\delta}\right)  \frac{1}{2}} $$
\end{theorem}

\begin{proof}
For some mechanism $\cM$ denote the privacy loss for all neighboring dataset $D$, $D'$ and all outcomes $r\in\cR$ as:
$$\cL_\cM(r) = \ln \left( \frac{ \pr{\cM(D)} = r)}{\pr{\cM(D')} = r)} \right)$$
And let the privacy loss for running $k$ mechanism be:
$$\cL_{\left( \cup_i^k \cM_i \right)} (r) = \sum_{i=1}^k \cL_{\cM_i}(r)$$
Since each $\cM_i$ is $\epsilon_i$-differentially private we have for all $r$ that $\cL_{\cM_i}(r) \leq \epsilon_i$ and, using lemma (ref here), $\Ex{ \cL_{\cM_i}(r) } \leq \epsilon_i(e^\epsilon_i-1)$.
The privacy loss is a function that depends on the randomized output of the private mechanisms $r_i$.
Now we apply Azuma's inequality in Lemma \ref{def:azuma}.
Let $r_1, \ldots, r_{i-1}$ be the output of mechanisms $\cM_1, \ldots \cM_{i-1}$ then for all $a, a' \in \cR$
$$\left| \Ex{\cL_{\left( \cup_i^k \cM_i \right)} | r_1, \ldots, r_{i-1}, r = a} - \Ex{\cL_{\left( \cup_i^k \cM_i \right)} | r_1, \ldots, r_{i-1}, r = a'} \right| \leq \epsilon_i   $$
Then by Azuma's:
\begin{equation*}
\begin{split}
\pr{\cL_{\left( \cup_i^k \cM_i \right)} (r_1, \ldots, r_k) \geq \Ex{\cL_{\left( \cup_i^k \cM_i \right)}} + t} \leq \exp\left( \frac{-2t^2}{\sum_{i=1}^k \epsilon_i^2}\right)
\end{split}
\end{equation*}
Letting $\Ex{\cL_{\left( \cup_i^k \cM_i \right)}} = \sum_{i=1}^k \epsilon_i(e^{\epsilon_i}-1)$ and $t = \sqrt{\left( \sum_{i=1}^k \epsilon_i^2 \right) \ln\left( \frac{1}{\delta}\right)  \frac{1}{2}} $
\begin{equation*}
\begin{split}
\pr{\cL_{\left( \cup_i^k \cM_i \right)} (r_1, \ldots, r_k) \geq \sum_{i=1}^k \epsilon_i(e^{\epsilon_i}-1) + \sqrt{\left( \sum_{i=1}^k \epsilon_i^2 \right) \ln\left( \frac{1}{\delta}\right)  \frac{1}{2}} } \leq \delta
\end{split}
\end{equation*}
\end{proof}

In this work we make the assumption that we have access to an optimization oracle such that, given a set of statistical linear queries, it outputs a data record from $\cX$ such that it approximatelly maximizes then answer score on the query set.
\begin{definition}[Approximate Linear Optimization Oracle] Given as input a set of $n$ statistical linear queries $\{q_i\}$ and a $d$-dimentional vector $\sigma$, an $\alpha$-approximate linear optimization oracle outputs
$$\hat{x} \in \argmin_{x\in\cX} \left\{ \sum_{i=1}^n q_i(x) -  \inner{x}{\sigma} \right\}$$
\end{definition}

\begin{definition}[Exponential Mechanism \cite{mcsherry2007mechanism}]
Given some database $D$, arbitrary range $\mathcal{R}$, and score function $S$, the exponential mechanism $\cM_E(D, S, \mathcal{R}, \eps)$ selects and outputs an element $r \in \mathcal{R}$ with probability proportional to $ \exp{\left( \frac{\varepsilon S(D, r)}{2 \Delta_S} \right)}$, where $\Delta_S$ is the sensitivity of $S$.
\end{definition}

\begin{lemma}[Theorem 3.12 in \cite{dwork2014algorithmic}]
The exponential mechanism $\mathcal{M}_E(x, S, \mathcal{R})$ is $(\varepsilon, 0)$-differentially private.
\end{lemma}
\begin{theorem}[Exponential Mechanism Error - Corollary 3.12 in \cite{dwork2014algorithmic}] \label{thm:exp-error}.
Fixing a database $x$, let ${OPT}_s(x)$ denote the max score function $s$. Then, with probability $1-\beta$ the error is bounded by:
%% $$ Pr\left[ u(\mathcal{M}_E(x, u, \mathcal{R})) \le {OPT}_u(x) - \frac{2\Delta u}{\varepsilon} \left( \ln{|\mathcal{R}|}+ t \right)\right] \le e^{-t} $$
$${OPT}_s(x) - s(\mathcal{M}_E(x, u, \mathcal{R})) \le  \frac{2 {GS}_s}{\varepsilon} \left( \ln{|\mathcal{R}|/\beta}\right) $$
\end{theorem}

\section{Missing Proof in Section ~\ref{sec:queryreleasegame}}

\subsection{Equilbrium of the Game}
Here we show that solving the query release game reduces to solving for the equilibrium of the zero sum game defined above. We make use von Neumann's minimax theorem which states that any zero-sum game has a unique value.
Let $\Delta (\cX)$ and $\Delta (\cQ)$ be the set of probability distributions over $\cX$ and $\cQ$.
According to von Neumann's minimax theorem, if each player plays from a probability distribution over their actions ($u\in\Delta(\cX)$ is the data player's action and $w\in\Delta(\cQ)$ is the query player's action), then:
$$\min_{u\in\Delta(\cX)} \max_{w\in\Delta(\cQ)} A(u, w) = \max_{w\in\Delta(\cQ)} \min_{u\in\Delta(\cX)} A(u, w) = v_A$$
where $$A(u, w) := \mathbb{E}_{x\sim u, q \sim w}A(x, q)$$ is the expected payoff and $v_A$ is the value of the game.
%This means that it does not matter whether the data player or query player plays first; in both cases their plays will still result in the same payoff $v_A$. Assumming best play from the opponent, each player can play an optimal strategy and the outcome of the game reaches an equilibrium.

\begin{definition}[$\alpha$-approximate equilibrium]\label{alpha-eq}
Let $\alpha > 0$. Let $A$ be the payoffs for a two player, zero-sum game with action sets $\cX, \cQ$. Then a pair of strategies $u^* \in \Delta (\cX)$ and $w^* \in \Delta (\cQ)$ form an $\alpha$-approximate mixed Nash equilibrium if
$$ A(u^*, w) \le v_a + \alpha \text{ and } A(u, w^*) \ge v_A - \alpha$$  for all strategies $u \in \Delta (\cX)$ and $w \in \Delta (\cQ)$. Note that $A(u^*, w)$ denotes the expected payoff for the best (minimizing) data response $u^*$ and $A(u, w^*)$ denotes the expected payoff for best (maximizing) query response $w^*.$
\end{definition}
Finally, the the following theorem shows that the $\alpha$-approximate nash equilibrium is a solution for the query release game:
\begin{theorem}\label{thm:gamesol} If $(u^*, w^*)$ is the $\alpha$-approximate equilibrium of a zero sum game between a data-player with action set $\cX$ and a query player with actions set $\cQ \cup \bar{\cQ}$ then for every $q\in\cQ \cup \bar{\cQ}$, we have
$$|q(u^*) - q(D)| \le \alpha$$
\end{theorem}
\textbf{Proof of Lemma~\ref{thm:gamesol}.}
\begin{proof}
We first show that the value of the game $v_A$ is zero. Let $\widehat{D} \in \Delta (\cX)$ be the normalized histogram distribution of $D$. We consider the following cases:

\begin{enumerate}
\item Any query $w$ and any data strategy over $\widehat{D}$ has zero payoff:
$$A(\widehat{D}, w) =  \mathbb{E}_{x\sim \hat{D}, q \sim w} [q(D)- q(X)] = 0.$$ Since the query player wants to maximize the payoff, it follows that the $v_A \le 0$:
$$v_A = \max_{w \in \Delta (\cQ)} \left[ \min_{u \in \Delta (\cX)} A(u, w) \right] \le \max_{w \in \Delta (\cQ)} A(\widehat{D}, w) = \max_{w \in \Delta (\cQ)} 0 = 0$$

\item For any data strategy $u$, the payoff of the query $q$ is equal to the negation of the payoff of the negated query $		\bar{q}$, i.e. $A(u, q) = - A(u, \bar{q})$:
$$A(u, \bar{q}) = \mathbb{E}_{x\sim u}[\bar{q}(D)-\bar{q}(x)] = \mathbb{E}_{x\sim u}[\bar{q}(x)-\bar{q}(D)] = -A(u, \bar{q}).$$
Because the query strategy places equal weight on $q$ and $\bar{q}$, the expected payoff $A(u, q)$ is zero. Since the data player minimizes the payoff, $v_a \ge 0$:
$$v_A = \min_{u \in \Delta (\cX)} \left[ \max_{w \in \Delta (\cQ)} A(u, w) \right] \ge \min_{u \in \Delta (\cX)} A(u, q) = \min_{u \in \Delta (\cX)} 0 = 0$$
\end{enumerate}

Thus $v_A = 0$ as desired. Let $(u^*, w^*)$ by the $\alpha$-approximate equilibrium. From the left inequality in Definition \ref{alpha-eq}, we know that when the data player plays $u^*$ and the query player plays $q$, the expected payoff is $A(u^*, w) = q(D) - q(u^*) \le \alpha$. Likewise, if the data player plays $u^*$ and the query player plays the negated query $\bar{q}$, the expected payoff is $A(u^*, \bar{q}) \le \alpha$ and $A(u^*, \bar{q}) = \bar{q}(D) - \bar{q}(u^*) = 1 - q(D) - (1-q(u^*)) = -q(D) + q(u^*)$. Thus, we have $q(D)-q(u^*) \ge - \alpha$ Therefore, we have $|q(u^*)-q(D)| \le \alpha$ as desired, so the setup of the $\alpha$-approximate equilibrium game satisfies the query release problem. Since the approximate data equilibrium $u^*$ is also the synthetic data, we just need to find $u^*$, which will then give us a query answer $q(u^*)$ that is accurate and private.
\end{proof}

The next theorem by Freund and Schapire shows that in a zero-sum game, if the two players maintains a distribution using a no-regret algorithm, then both of the players' actions converge to an $\alpha$-approximate equilibrium.
\begin{theorem}[Freund and Schapire\cite{freund1996game}]\label{thm:freund}
\label{theorem:FreundSchapire}
Let $\alpha>0$, and let $A(i,j) \in [-1,1]^{m \times n}$ be the payoff matrix for a zero-sum game. Suppose the first player uses a no-regret strategy over their actions to play distributions $p^1, \ldots, p^T$ and obtains average regret $R_1(T)$, while the second player plays approximate best responses $x^1, \ldots, x^T$ with regret $R_2(T)$. If $T$ is selected such that $R_1(T) = R_2(T)$, then the empirical distributions
$$\frac{1}{T}\sum_{t=1}^T p^t \textit{ and } \frac{1}{T}\sum_{t=1}^T x^t$$
form an $(R_1(T) + R_2(T))$-approximate Nash equilibrium.
\end{theorem}

%From theorem \ref{thm:freund}, it follows that to achieve an $\alpha$-approximate Nash equilibrium, the data player and the query player must both play algorithms with known regret bounds. Because FTPL and EM have known regret bounds as discussed in Section \ref{prelim:no-regret-alg}, the data player plays a no-regret FTPL and the query player best responds with Exponential Mechanism.
From theorem \ref{thm:freund} and \ref{thm:gamesol}, it follows that having the data player and the query player playing algorithms with known regret bounds leads to a solution to the query release game. In the next section we introduce a general framework for analysing private no-regret dynamics.\cite{dwork2006differential}.

\section{Missing Proof in Section ~\ref{sec:noregretdynamics}}
\textbf{Proof of Theorem~\ref{thm:frameworkprivacy}.}
\begin{proof}
By the advanced composition theorem, running a composition of $k$ $\varepsilon_0$-private mechanisms is $(\varepsilon, \delta)$-private for $$\varepsilon = \sqrt{2k \log{(1/\delta)}}\varepsilon_0 + k\varepsilon_0(\exp{(\varepsilon_0)}-1) $$

The privacy cost of each round is $\varepsilon_0$ and there are $k = T$ rounds. We plug in $\varepsilon_0$ and $k$ accordingly into the advanced composition theorem to get
$$\varepsilon = \sqrt{2T \log{(1/\delta)}}\varepsilon_0 + T\varepsilon_0(\exp{(\varepsilon_0)}-1).  $$
Since $\exp{(\varepsilon_0)} \le 1 + 2 \varepsilon_0$ for $0 < \varepsilon_0 < 1$, we can simplify the expression to get
$\epsilon \le  \sqrt{2T \log{(1/\delta)}}\varepsilon_0 + 2T{\varepsilon_0}^2$. Solving for $\varepsilon_0$ we find that

\begin{equation*}
\begin{split}
\varepsilon_0 &= \frac{\sqrt{2T\log{(1/\delta)} + 8T\varepsilon} - \sqrt{2T\log{(1/\delta)}}}{4T} \\
& = \frac{1}{4T} \cdot \frac{8T\varepsilon}{\sqrt{2T\log{(1/\delta)} + 8T\varepsilon} + \sqrt{2T\log{(1/\delta)}}} \\
& = \frac{2\varepsilon}{\sqrt{2T\log{(1/\delta)}} \left( 1 + \sqrt{1 + \frac{4\varepsilon}{\log{(1/\delta)}}} \right)} \\
& =  \frac{\varepsilon}{\frac{\sqrt{2}}{2} \left( 1 + \sqrt{1 + \frac{4\varepsilon}{\log{(1/\delta)}}} \right) \sqrt{T\log{(1/\delta)}}} \\
& < \frac{\varepsilon}{\frac{\sqrt{2}}{2} (1+1) \sqrt{T\log{(1/\delta)}}} \\
\end{split}
\end{equation*}

Thus we get $\varepsilon_0$ as desired.
\end{proof}

%\section{Missing algorithms in Section~\ref{sec:accuracy}}
Next we describe the details of algorithm \fem and the accuracy guarantee proof.
% \begin{algorithm}[H]
% \label{algorithm:fem}
% \SetAlgoLined
% \KwIn{A dataset $D$, A queryset $\cQ$}
% $s  = \frac{8 \log{(4T/\beta)}}{\alpha^2}$ \;
% $\eta = \sqrt{\frac{1 + \log{d}}{125dT}}$ \;
% 	Let $\sigma_j^t \sim Exp(\eta) $\;
% 	Sample $s$ data values $\{ x_j^t \}$ according to $\argmax_x \left \{ \sum_{i=1}^{t-1} q_i(x) - x \sigma_j^t \right \}$\;
% \KwOut{$ \widehat{D^t} := \{ x_1^t, x_2^t, \ldots , x_s^t \}$}
% \caption{\fem}
% \end{algorithm}
\begin{algorithm}[h]
\begin{algorithmic}
\caption{\fem}
\label{alg:appex:fem}
\INPUT A dataset $D$, A queryset $\cQ$
\STATE $s  = \frac{8 \log{(4T/\beta)}}{\alpha^2}$
\STATE $\eta = \sqrt{\frac{1 + \log{d}}{125dT}}$
\STATE Let $\sigma_j^t \sim Exp(\eta) $
\STATE Sample $s$ data values $\{ x_j^t \}$ according to $\argmax_x \left \{ \sum_{i=1}^{t-1} q_i(x) - x \sigma_j^t \right \}$
\OUTPUT $ \widehat{D^t} := \{ x_1^t, x_2^t, \ldots , x_s^t \}$\end{algorithmic}
\end{algorithm}

The accuracy proof proceeds in two steps. First we show that the sample distribution $\widehat{D^t}$ played by the data player is close the true distribution $D^t$ and we show that the query player plays an approximate best response. Then, by theorem \ref{theorem:FreundSchapire}, we show that algorithm \ref{algorithm:fem} finds an approximate equilibrium.

We use Chernoff bound.
\begin{lemma}[Chernoff bound \cite{dwork2014algorithmic}] \label{def:chernoff}
Let $X_1, \ldots, X_m$ be i.i.d random variables such that $0 \le X_i \le 1$ for all $i$. Let $S = \frac{1}{m} \sum_{i=1}^m X_i$ denote their mean and let $\mu = \mathbb{E}[S]$ denote their expected mean. Then,
$$\pr{|S - \mu| > T ] \le 2 \exp{(-2mT^2)}}$$
\end{lemma}

\begin{lemma}\label{lemma:datasampling}
Let $\beta \in (0, 1)$ and let $D^t$ be the true distribution over $\cX$. Suppose we draw
$$s  = \frac{8 \log{(4T/\beta)}}{\alpha^2}$$ samples $\{ x_i^t \}$ from $D^t$ to form $\widehat{D^t}$. Then with probability at least $1 - \beta / 2$, we have $$\left|\frac{1}{s} \sum_{i=1}^s q(x_i^t)- q(D^t)\right| < \frac{\alpha}{4}$$ for all $0 \le t \le T$
\end{lemma}

\begin{proof}
For any fixed $t$, note that $\frac{1}{s} \sum_{i=1}^s q(x_i^t)$ is the average of the random variables $q(x_1^t), q(x_2^t), \ldots, q(x_s^t)$. Also $\mathbb{E}[q(x^t)] = q(D^t)$ for all $0 \le t \le T$. Thus by the Chernoff bound and our choice of $s$,
$$\pr{\left|\frac{1}{s} \sum_{i=1}^s q(x_i^t)- q(D^t)\right| > \frac{\alpha}{4}} \le 2\exp{(-s \alpha^2 /8)} = \beta/2T. $$ A union bound over all $T$ rounds gives a total fail probability of at most $\beta/2$ as desired.
\end{proof}

\begin{lemma}[Data Player's Regret]\label{lemma:data-regret}
Given that the data player plays the distributions $\widehat{D^1}, \widehat{D^2} \ldots \widehat{D^T}$, the data player achieves an average regret bound of
$$\frac{1}{T}\sum_{t=1}^T A(\widehat{D^t}, q^t) - \min_{x \in \cX} \frac{1}{T} \sum_{t=1}^T A(x, q^t) \le  \frac{\alpha}{4} + (125 + 5\sqrt{5})\sqrt{\frac{d^3(1+\log {d)}}{T}} $$
for all $T$ rounds with probability at least $1- \beta/2$.
\end{lemma}

\begin{proof}
We calculate the average error per round of the data and query player to find the value of $\alpha$, the additive error of each query, with probability at least $1-\beta$ using Theorem \ref{thm:freund}.

Because $\widehat{D^t}$ approximates $D^t$ with probability at least $1-\beta/2$, we calculate the average regret per round when the data player plays with the true distribution $D^t$.
We assume that our oracle is efficient so $\alpha' = 0$. Since the dimension of the perturbation is the dimension of the dataset, $d = \log{\cX}$. We also have $D = 1$ and $L = 1$. From the FTPL regret bound \cite{gonen2018learning}, since $ \mathbb{E}_\sigma \left[ \sum_{t=1}^{T} A(x^t, q^t) - \min_{x \in \cX} \sum_{t=1}^{T} A(x^t, q^t) \right] =  \sum_{t=1}^{T} A(D^t, q^t) - \min_{x\in \cX} \sum_{t=1}^{T} A(x, q^t)$, the average regret per round for the data player playing the true distribution $D^t$ has the following bound:

$$\frac{1}{T}\sum_{t=1}^T A(D^t, q^t) - \min_{x \in \cX} \frac{1}{T} \sum_{t=1}^T A(x, q^t)  \le 125 \eta d^2+ \frac{(1+\log{d}) d}{T\eta} $$.

 From Lemma \ref{lemma:datasampling}, we know that with probability at least $1-\beta/2$, the average error per round of sample distribution $\widehat{D^t}$ from the true distribution $D^t$ is $\alpha/4$. Hence, with probability at least $1-\beta/2$, the average regret per round for the data player playing the sample distribution $\widehat{D^t}$ is
$$\frac{1}{T}\sum_{t=1}^T A(\widehat{D^t}, q^t) - \min_{x \in \cX} \frac{1}{T} \sum_{t=1}^T A(x, q^t)   \le \frac{\alpha}{4} + 125 \eta d^2+ \frac{(1+\log{d}) d}{T\eta}$$

Setting $\eta = \sqrt{\frac{1 + \log{(d)}}{125Td}}$, we have
%and since $\min_{D \in \Delta(\cX)}\sum_{t=1}^T A(D, q^t) = \min_{x}\sum_{t=1}^T A(x, q^t)$, we have
$$\frac{1}{T}\sum_{t=1}^T A(\widehat{D^t}, q^t) -\min_{x \in \cX}  \frac{1}{T} \sum_{t=1}^T A(x, q^t)   = \frac{\alpha}{4} + (125 + 5\sqrt{5})\sqrt{\frac{d^3(1+\log {(d))}}{T}}$$ as desired.
\end{proof}

We next calculate the upper bound of the average error per round for the query player playing the exponential mechanism with probability at least $1-\beta/2$.

\begin{lemma}[Query Player's Regret]\label{lemma:query-regret}
The query player achieves an average regret bound of
$$\max_{q \in \cQ} \frac{1}{T} \sum_{t=1}^T A(\widehat{D^t}, q^t) - \frac{1}{T} \sum_{t=1}^T A(\widehat{D^t}, q^t) \le \frac{2/n}{\varepsilon_0} \ln{\left(2T|\mathcal{Q}|/\beta\right)} = \frac{2\sqrt{2}}{n\varepsilon}\sqrt{T\log{(1/\delta)}}\ln{\left( \frac{2T|\cQ|}{\beta} \right)}$$
for all $T$ rounds with probability $1-\beta/2$.
\end{lemma}

\begin{proof}
Since the sensitivity of the query player's score function $GS_s$ is $1/n$, then with probability $1-\beta/2T$ the error for each is round is at most $\frac{2/n}{\varepsilon} \ln{\left(2T|\mathcal{Q}|/\beta\right)}$ by Theorem \ref{thm:exp-error}. Applying union bound over $T$ rounds, with probability $1-\beta/2$ the query player's average regret for $T$ rounds is

$$\max_{q \in \cQ} \frac{1}{T} \sum_{t=1}^T A(\widehat{D^t}, q^t) - \frac{1}{T} \sum_{t=1}^T A(\widehat{D^t}, q^t) \le \frac{2/n}{\varepsilon_0} \ln{\left(2T|\mathcal{Q}|/\beta\right)} = \frac{2\sqrt{2}}{n\varepsilon}\sqrt{T\log{(1/\delta)}}\ln{\left( \frac{2T|\cQ|}{\beta} \right)}$$
\end{proof}

Our final accuracy guarantee follows.\\
\textbf{Proof of Theorem~\ref{thm:femaccuracy}.}
\begin{proof}
From Lemma \ref{lemma:data-regret} and Lemma \ref{lemma:query-regret}, let $R_D(T)$ and $R_Q(T)$ be the upper bounds for the average error of the data and query player respectively with probability at least $1-\beta/2$. Then, with probability at least $1-\beta$ due to the union bound over 2 events, $\alpha$ is the average regret for all rounds by Theorem \ref{thm:freund}:
\begin{equation*}
\begin{split}
\alpha &= R_D(T) + R_Q(T) \\
& = \frac{\alpha}{4} + (125 + 5\sqrt{5})\sqrt{\frac{d^3(1+\log {d})}{T}} + \frac{2\sqrt{2}}{n\varepsilon}\sqrt{T\log{(1/\delta)}}\ln{\left( \frac{2T|\cQ|}{\beta} \right)} \\
\end{split}
\end{equation*}
Setting $T = \frac{125+5\sqrt{5}}{2\sqrt{2}} \frac{n\varepsilon \cdot [d^3 (1+\log{d})]^{1/2}}{\log{\frac{2|\cQ|}{\beta}}\log^{1/2}{(1/\delta)}} $, we have
\begin{equation*}
\begin{split}
\frac{3\alpha}{4} &< 2(250\sqrt{2} + 10\sqrt{10})^{1/2}\frac{\left[ d^3(1+\log{d}\right]^{1/4} \log^{1/4}(1/\delta)}{n^{1/2}\varepsilon^{1/2}} \left[2\log^{1/2}\left(\frac{2|\cQ|}{\beta}\right) + \log^{-1/2}\left(\frac{2|\cQ|}{\beta}\right) \ln{T} \right]\\
\alpha &= O \left( \frac{d^{3/4} \cdot \log^{1/4}(1/\delta) \log^{1/2}\left( \frac{2|\cQ|}{\beta} \right)} {n^{1/2} \varepsilon^{1/2}} \cdot \text{polylog}\left(d, n, \varepsilon, \log(1/\delta), \log|\cQ|, \log{(1/\beta)} \right)\right)
\end{split}
\end{equation*}
\end{proof}

%%%%%
%% sepFEM
\begin{definition} A set $\sepQ$ is a small-separator for queries $\cQ$ if for any two distinct records $x,x'\in \cX$, there exist $q \in \sepQ$ such that  $q(x) \neq q(x')$.
\end{definition}

% \SetKwInOut{Parameter}{Parameters}
% \begin{algorithm}[H]
% \label{algorithm:sep-fem}
% \SetAlgoLined
% \KwIn{A dataset $D$, the $t-1$ queries $\{q_1, \ldots, q_{t-1}\}$, A queryset $\cQ$ with small separator set $\sepQ$ }
% \Parameter{Laplace noise parameters $\eta$, The number of samples $s$}
% %$T = \frac{125+5\sqrt{5}}{2\sqrt{2}} \frac{n\varepsilon \cdot [d^3 (1+\log{d})]^{1/2}}{\log^{1/2}{(1/\delta)}} $\;
% %$\varepsilon_0 = \frac{\varepsilon}{\sqrt{2T \log{(1/\delta)}}}$ \;
% %$s  = \frac{8 \log{(4T/\beta)}}{\alpha^2}$ \;
% %$\eta = \sqrt{\frac{1 + \log{d}}{125dT}}$ \;
% %Let $\tilde{q} \leftarrow \{q_1, \ldots, q_{t-1}\}$\;
% %Let $M \leftarrow |\sepQ|$\;
% Let $\tilde{q} \leftarrow \sepQ$ and $M \leftarrow |\sepQ|$\;
% \For{$i \gets 1 $ \KwTo $s$}{
% 	Sample noise vector $\sigma \sim \Lap(\eta)^M$\;
% 	Get $x_i \in \argmax_x \left \{ \sum_{j=1}^{t-1} q_j(x) + \sum_{j=1}^M \sigma_j \tilde{q}_j(x) \right \}$\;
% }
% %Generate $s$ noise vectors $\{\sigma_i \}$ from distribution $\Lap(\eta)^M$\;
% %Sample $s$ data values $\{ x_i \}$ according to $\argmax_x \left \{ \sum_{q\in\tilde{q}} q(x) - x \sigma_i \right \}$	\;
% \KwOut{$\widehat{D} = \{ x_1, x_2, \ldots , x_s \}$}
% \caption{\sfem}
% \end{algorithm}

%\begin{theorem}[Separator FTPL + EM Accuracy]
%With probability at least $1-\beta$, the algorithm with separator FTPL finds a synthetic database that answers all queries in $\cQ$ with additive error $$\alpha = O \left( \frac{d^{5/8} \log^{1/4} |\cQ| \cdot \log^{1/2}(1/\delta) \log^{1/2}(1/\beta)} {n^{1/2} \varepsilon^{1/2}} \right)$$
%\end{theorem}

\begin{algorithm}[h]\label{alg:sep-fem}
\begin{algorithmic}
\caption{\sfem}
\REQUIRE Laplace noise parameters $\eta$, The number of samples $s$
\INPUT A dataset $D$, the $t-1$ queries $\{q_1, \ldots, q_{t-1}\}$, A queryset $\cQ$ with small separator set $\sepQ$
\STATE Let $\tilde{q} \leftarrow \sepQ$ and $M \leftarrow |\sepQ|$
\FOR{$i \gets 1 $\textbf{to} $s$}
	\STATE Sample noise vector $\sigma \sim \Lap(\eta)^M$\;
	\STATE Get $x_i \in \argmax_x \left \{ \sum_{j=1}^{t-1} q_j(x) + \sum_{j=1}^M \sigma_j \tilde{q}_j(x) \right \}$\;
\ENDFOR
\OUTPUT $ \widehat{D^t} := \{ x_1^t, x_2^t, \ldots , x_s^t \}$
\end{algorithmic}
\end{algorithm}

\textbf{Proof of Theorem~\ref{thm:sepfemaccuracy}.}
\begin{proof}
%From Lemma \ref{lemma:data-regret} and Lemma \ref{lemma:query-regret}, let $R_D(T)$ and $R_Q(T)$ be the upper bounds for the average error of the data and query player respectively with probability at least $1-\beta/2$.
Setting $\eta = (5/2)^{1/2} d^{1/4} T^{-1/2}$, the data player's average regret for all $T$ rounds is $R_D(T) = 4\sqrt{10} d^{5/4} T^{-1/2}$ and the average regret for the query player is $R_Q(T)$ given by lemma \ref{lemma:query-regret}.
If $T =  \frac{2\sqrt{5} d^{5/4} n\varepsilon }{\log^{1/2}{(1/\delta)} \log{\left( \frac{2|\cQ|}{\beta}\right)}} $, then, by union bound and by Theorem \ref{thm:freund}, with probability at least $1-\beta$,  the accuracy of \sfem is:
\begin{equation*}
\begin{split}
\alpha &= R_D(T) + R_Q(T) \\
& =  4\sqrt{10}d^{5/4}T^{-1/2}+ \frac{2\sqrt{2}}{n\varepsilon}\sqrt{T\log{(1/\delta)}}\ln{\left( \frac{2T|\cQ|}{\beta} \right)} \\
\end{split}
\end{equation*}
%Setting $T =  \frac{2\sqrt{5} d^{5/4} n\varepsilon }{\log^{1/2}{(1/\delta)} \log{\left( \frac{2|\cQ|}{\beta}\right)}} $, we have
Plugging in the value of $T$,
\begin{equation*}
\begin{split}
\alpha &= \frac{ 8\sqrt[4]{5} d^{5/8}\log^{1/4}{(1/\delta)}\log^{1/2}{\left( \frac{2T|\cQ|}{\beta}\right)}}{n^{1/2}\varepsilon^{1/2}}\\
\end{split}
\end{equation*}
\end{proof}

%\section{Missing algorithms in Section~\ref{sec:rs}}
\section{\dqrs: \dq with Rejection Sampling}

In this section, we present an improvement from the \DQ algorithm \cite{gaboardi2014dual}. In \DQ, the query player maintains a distribution over queries using Multiplicative Weights. But the algorithm can't directly release the distribution $\cQ^t$ proposed by MW during round $t$ because it depends on the private data. Instead, for each round $t$, it takes $s$ samples from $\cQ^t$ to form an estimate distribution $\widehat{\cQ^t}$. The data player then best-responds against $\widehat{\cQ^t}$. Our algorithm \dqrs improves the sampling step of \DQ. The basic idea is to apply the rejection sampling technique to generate a sample from $\cQ^t$ using samples obtained from the distribution in the previous round, i.e., $\cQ^{t-1}$. We show that by taking fewer samples from $\cQ^t$ for each round $t$, we use less of the privacy budget. The result is that the algorithm operates
for more iterations and obtains better performance.

\begin{theorem}
  \label{thm:rsprivacy}
  \dq with rejection sampling (Algorithm \ref{alg:dqrs}) takes in a private dataset $D \in \cX^n$ and makes $T=O\left(\frac{\log|\cQ|}{\alpha^2}\right)$ queries to an optimization oracle and outputs a dataset $\tilde{D}=(x^1, \cdots, x^T)\in \cX^T$ such that, with probability at least $1-\beta$, for all $q \in \cQ$ we have $|q(\tilde{D})-q(D)|\le\alpha$. The algorithm is $\rho$-CDP for $$\rho=O\left( \frac{\log(|\cX|T/\beta) \cdot \log^3(|\cQ|)}{n^2 \alpha^5}\right).$$
\end{theorem}

In contrast, \dq (\emph{without} rejection sampling) obtains the same result except with $$\rho = O\left(\frac{\log(|\cX|T/\beta) \cdot \log^3(|\cQ|)}{n^2 \alpha^7}\right).$$

To obtain $(\varepsilon,\delta)$-differential privacy, it suffices to have $\rho$-CDP for $\rho=\Theta(\varepsilon^2/\log(1/\delta)$. Thus the guarantee of Theorem \ref{thm:rsprivacy} can be rephrased as the sample complexity bound $$n=O\left(\frac{\log^{1.5}(|\cQ|) \cdot \sqrt{ \log(|\cX|T/\beta) \cdot \log(1/\delta)}}{\alpha^{2.5} \varepsilon}\right)$$ to obtain $\alpha$-accurate synthetic data with probability $1-\beta$ under $(\varepsilon,\delta)$-differential privacy.

% \SetKwInput{init}{Initialize}
% \SetKwInOut{Parameter}{Parameters}
%
% \begin{algorithm}[H]
% \label{algorithm:rs}
% \SetAlgoLined
% \Parameter{Target accuracy $\alpha \in (0,1)$, target failure probability $\beta \in (0,1)$}
% \KwIn{dataset $D$, and linear queries $q_1, \ldots, q_k \in \cQ$ }
% \init{Let $\cQ = \bigcup_{i=1}^k q_i \cup \bar{q_i}$, and $Q^1$ a uniform distribution on $\cQ$}
% %\KwOut{Sample $y_1, \ldots, y_s$}
%
% Set $T  = \frac{16 \log |\cQ|}{\alpha^2}$, $\eta = \frac{\alpha}{4}$, $\gamma_t = \frac{1}{2t^{2/3}}$, $s = \frac{48 \log \left({3 |\cX| T}/{\beta} \right)}{\alpha^2}$, and $\tilde{s}_t = (2\gamma_t+4\eta) s$.
%
% Construct sample $S_1$ of $s$ queries $\{q_i\}$ from $\cQ$ according to $\cQ^1$\;
% \For{$t \gets 1 $ \KwTo $T$}{
% 	%Sample $s$ queries $\{q_i\}$ using rejection sampling. with $M=\exp(\eta)$\;
%
% 	Let $\tilde{q} = \frac{1}{s}\sum_{q \in S_t} q$\;
% 	Find $x^t$ with $A_D(x^t, \tilde{q}) \geq \max_{x} A_D(x, \tilde{q}) - \alpha/4$\;
% 	\For{$q \in \cQ$}{
% 		$\hat{\cQ}_q^{t+1} :=e^{-\eta-\gamma_t} \cdot  \exp\left(-\eta A_D (x^t, q) \right)\cQ_q^{t}$\;
% 	}
% 	Normalize $\hat{\cQ}^{t+1}$ to obtain $\cQ^{t+1}$\;
% 	Construct $S_{t+1}$ as follows\;
% 	\For{$q \in S_t$}{
% 		Add $q$ to $S_{t+1}$ with probability $\hat{\cQ}^{t+1}/\cQ^{t}$\;
% 		Add $\tilde{s}_t$ independent fresh samples from $Q^{t+1}$ to $S_{t+1}$.\;
% 		If $|S_{t+1}|>s$, discard elements at random so that $|S_{t+1}|=s$.\;
% 		%$\cQ_q^{t+1} := \exp\left(-\eta A_D (x^t, q) \right)\cQ_q^{t}$\;
% 	}
% }
% \caption{Rejection Sampling Dualquery}\label{alg:dqrs}
% \end{algorithm}

\begin{algorithm}[h]\label{alg:dqrs}
\begin{algorithmic}
\caption{Rejection Sampling Dualquery}
\REQUIRE Target accuracy $\alpha \in (0,1)$, target failure probability $\beta \in (0,1)$
\INPUT dataset $D$, and linear queries $q_1, \ldots, q_k \in \cQ$
\STATE Set $T  = \frac{16 \log |\cQ|}{\alpha^2}$, $\eta = \frac{\alpha}{4}$
\STATE $s = \frac{48 \log \left({3 |\cX| T}/{\beta} \right)}{\alpha^2}$
% , and
\STATE Construct sample $S_1$ of $s$ queries $\{q_i\}$ from $\cQ$ according to $\cQ^1$
\FOR{$t \gets 1 $ \textbf{ to } $T$}
	% \STATE Add $q$ to $S_{t+1}$ with probability $\hat{\cQ}^{t+1}/\cQ^{t}$\;
	\STATE Let $\tilde{q} = \frac{1}{s}\sum_{q \in S_t} q$\;
	\STATE Find $x^t$ with $A_D(x^t, \tilde{q}) \geq \max_{x} A_D(x, \tilde{q}) - \alpha/4$\;
  \STATE Let $\gamma_t = \frac{1}{2t^{2/3}}$
	\FORALL{$q \in \cQ$}
		\STATE $\hat{\cQ}_q^{t+1} :=e^{-\eta-\gamma_t} \cdot  \exp\left(-\eta A_D (x^t, q) \right)\cQ_q^{t}$\;
	\ENDFOR

	\STATE Normalize $\hat{\cQ}^{t+1}$ to obtain $\cQ^{t+1}$
  \STATE Construct $S_{t+1}$ as follows
  \STATE Let $\tilde{s}_t = (2\gamma_t+4\eta) s$ and add $\tilde{s}_t$ independent fresh samples from $Q^{t+1}$ to $S_{t+1}$
	\FORALL{$q \in S_t$}
		\STATE Add $q$ to $S_{t+1}$ with probability $\hat{\cQ_q}^{t+1}/\cQ_q^{t}$
		\STATE If $|S_{t+1}|>s$, discard elements at random so that $|S_{t+1}|=s$
		%$\cQ_q^{t+1} := \exp\left(-\eta A_D (x^t, q) \right)\cQ_q^{t}$\;
	\ENDFOR
\ENDFOR
\OUTPUT Sample $y_1, \ldots, y_s$
\end{algorithmic}
\end{algorithm}

\begin{lemma} \label{lem:good-samples}
The subroutine which accepts $q$ with probability $\hat{Q}^{t+1}_q /  Q^t_q = e^{-\eta-\gamma_t} \cdot \exp(-\eta A_D(x^t, q) )$ is $\eps$-differentially private for $\eps = \max\left\{\eta / n, \eta/\gamma_t n\right\}$.
\end{lemma}
%\textbf{Proof of Lemma~\ref{lem:good-samples}.}
\begin{proof}
Note that $0 < p:=\hat{Q}^{t+1}_q /  Q^t_q = e^{-\eta-\gamma_t} \cdot \exp(-\eta A_D(x^t, q) ) \le e^{-\gamma_t} < 1$. In particular, the probability is well-defined.

We compute the ratio between the probabilities that $q$ is accepted under executions of the algorithm on neighboring datasets $D, D'$ for fixed choices of the best responses $x^1, \dots, x^t$. This ratio is given by
\[
\frac{p}{p'}=\frac{\hat{Q}^{t+1}_q[D]}{Q^t_q[D]} \cdot \frac{Q^{t}_q[D']}{\hat{Q}^{t+1}_q[D']}
= \frac{\exp(-\eta A_D(x^t, q))}{\exp(-\eta A_{D'}(x^t, q))}
\le e^{\eta / n}.
\]
Similarly, we evaluate the ratio of the probabilities that $q$ is \emph{not} accepted under executions of the algorithm on $D$ and $D'$:
Since $p' \le e^{-\gamma_t}$ and $p/p' \ge e^{-\eta/n}$, we have
\[
\frac{1-p}{1-p'} = 1 + \frac{1}{1/p'-1}\left(1-\frac{p}{p'}\right) \le 1 + \frac{1- e^{-\eta/n}}{e^{\gamma_t}-1} \le 1 + \frac{\eta/n}{\gamma_t} \le e^{\eta/\gamma_t n},
\]
as required. %For the final inequality to hold we need $\varepsilon \ge \log\left(1 + \frac{1- e^{-\eta/n}}{e^{\gamma_t}-1} \right)$, for which $\varepsilon \ge \eta/\gamma_t n$ suffices.
%$$\frac{1}{e^{\gamma}-1} =  \frac{e^{-\gamma}}{1-e^{-\gamma}}  \le \frac{e^{\varepsilon}-1}{1- e^{-\eta/n}}$$ $$e^\gamma  \ge 1+\frac{1- e^{-\eta/n}}{e^{\varepsilon}-1}$$
\end{proof}

Bad samples also incur privacy loss from sampling from the distribution $Q^t$. Just as in~\cite{gaboardi2014dual}, we use the fact that this step can be viewed as an instantiation of the exponential mechanism with score function $\sum_{i = 1}^{t-1}(q(D) - q(x^i))$ to obtain:
\begin{lemma} \label{lem:bad-samples}
Sampling from $Q^{t}$ is $\eps$-differentially private for $\eps = 2\eta(t-1)/n$.
\end{lemma}

\textbf{Proof of Privacy for Theorem~\ref{thm:rsprivacy}.}
\begin{proof}

%By Lemma~\ref{lem:num-bad} and a union bound, the number of bad samples in any given round $t = 1, \dots, T$ is at most $(1-e^{-2\eta-\gamma})s + \sqrt{\frac12 s\log(2T/\delta)}$ with probability $\delta/2$. Conditioning on this event,
Each round $t$ incurs privacy loss from $s$ invocations of a $(\eta/\gamma_t n)$-differentially private algorithm (rejection sampling, Lemma~\ref{lem:good-samples}), and $\tilde{s}_t$ invocations of a $(2\eta(t-1)/n)$-differentially private algorithm (Lemma~\ref{lem:bad-samples}).
Since $\varepsilon$-differential privacy implies $\frac12\varepsilon^2$-CDP \cite{BunS16}, we have (by composition) that round $t$ is $\rho_t$-CDP for $$\rho_t = \frac{\eta^2}{2\gamma_t^2n^2}s + \frac{2\eta^2(t-1)^2}{n^2}\tilde{s}_t = \frac{\eta^2s}{n^2}\left(\frac{1}{2\gamma_t^2} + 2(t-1)^2 \cdot (2\gamma_t+4\eta)\right) \le \frac{\eta^2s}{n^2}\left(4t^{4/3} + 8\eta t^2\right).$$
Composing over rounds $t=1 \cdots T$ yields $\rho=O\left( \frac{\log(|\cX|T/\beta) \cdot \log^{2+1/3}(|\cQ|)}{n^2 \alpha^{4+2/3}} + \frac{\log(|\cX|T/\beta) \cdot \log^3(|\cQ|)}{n^2 \alpha^5}\right)$, as required.

\end{proof}

\subsection*{Accuracy}

The accuracy analysis follows that of of \dq, together with the following claims showing that the rejection sampling process simulates the collection of independent samples in the \dq algorithm.

\begin{lemma}\label{lem:rs-dist}
Let $P$ and $Q$ be probability distributions over $\cQ$, and let $M \ge \max_{q \in \cQ} P_q / Q_q$. Sample an element of $\cQ$ as follows. Sample $q$ according to $Q$, and accept it with probability $P_q / (M\cdot Q_q)$. If $q$ is not accepted, sample $q$ according to $P$. Then the resulting element is distributed according to $P$.
\end{lemma}
%\textbf{Proof of Lemma~\ref{lem:rs-dist}.}
\begin{proof}
The total probability of sampling $q$ according to this procedure is given by
\begin{align*}
Q_q \cdot \frac{P_q}{M \cdot Q_q} + P_q \cdot \sum_{q' \in \cQ} Q_{q'} \cdot \left(1 - \frac{P_{q'}}{M \cdot Q_{q'}} \right) &= P_q \cdot \left(\frac{1}{M} + \sum_{q' \in \cQ} \left(Q_{q'} - \frac{P_{q'}}{M} \right) \right) \\
&= P_q \cdot \left(\frac{1}{M} +  \left(1 - \frac{1}{M} \right) \right) \\
&= P_q.
\end{align*}
\end{proof}

\begin{lemma}\label{lem:rs-bound}
For any given round $t$, the probability that more than $\tilde{s}_t$ samples are rejected is at most $(e/4)^{\tilde{s}_t} \le \frac{\beta}{3T}$.
\end{lemma}
%\textbf{Proof of Lemma~\ref{lem:rs-bound}.}
\begin{proof}
The probability that any given sample is rejected is $1-\hat{Q}^{t+1}_q /  Q^t_q = 1-e^{-\eta-\gamma_t} \cdot \exp(-\eta A_D(x^t, q) ) \le 1-e^{-2\eta-\gamma_t} \le 2\eta+\gamma_t = \frac{\tilde{s}_t}{2s}$. (In particular, $\tilde{s}_t$ is at least twice the expected number of rejected samples.) The set of $s$ samples is rejected independently.
By a multiplicative Chernoff bound, the probability that more than $\tilde{s}_t$ samples are rejected is at most $(e/4)^{\tilde{s}_t}$. Note that $\tilde{s}_t \ge 4\eta s = \frac{48}{\alpha} \log\left(\frac{3|\cX|T}{\beta}\right)$. Thus $(e/4)^{\tilde{s}_t} \le \left(\frac{\beta}{3|\cX|T}\right)^{18/\alpha} \le \frac{\beta}{3T}$.
\end{proof}

Together Lemmas \ref{lem:rs-dist} and \ref{lem:rs-bound} show that, with high probability, at each round $t$, the set $S_t$ is distributed as $s$ independent samples from $\cQ^t$. Given this, the rest of the proof follows that of the original \dq.

%%%%%%%%%%%%%%%%%%%%%%%%%%%%
%% Accuracy of DQRS
%%%%%%%%%%%%%%%%%%%%%%%%%%%%
\textbf{Proof of Accuracy for Theorem~\ref{thm:rsprivacy}.}
\begin{proof}
For each round $t$, by Hoeffding's bound and Lemma \ref{lem:rs-bound} and a union bound over $\cX$, with probability at least $1-\frac{\beta}{T}$, we have $$\forall x \in \cX \qquad \left|\frac{1}{s} \sum_{q \in S_t} q(x) - \underset{q \leftarrow \cQ^t}{\mathbb{E}}\left[ q(x) \right]\right| \le \frac{\alpha}{4}.$$
By a union bound over the $T$ rounds we have that the above holds for all $t \in [T]$ with probability at least $1-\beta$.

By assumption, in each round $t$, our oracle returns $x^t$ that is an $\alpha/4$-approximate best response to the uniform distribution over $S_t$. Thus, with high probability, the sequence $x^1, \cdots, x^T$ are $\alpha/2$-approximate best responses to the distributions $Q^1, \cdots, Q^t$. Since the distributions are generated by multiplicative weights, we have that this is an $\alpha$-approximate equilibrium. Hence the uniform distribution over $x^1, \cdots, x^T$ is an $\alpha$-accurate synthetic database for $D$.
\end{proof}
